# Supplementary material for: Constraints on Lightly Ionizing Particles from CDMSlite
Source: arXiv:2011.09183 ancillary file (2022-02-19)
Supplement: Supplementary file 1 [file CDMSliteRun2aLIPsSearch_DataRelease_v1.3.pdf]

# Data Release for CDMSlite Run 2 Period 1 LIP-search Analysis

SuperCDMS Collaboration

January 31, 2022

This document describes the public release of the data relevant to the SuperCDMS publication titled “Constraints on Lightly Ionizing Particles from CDMSlite” [1]. The upper limits on intensity of LIPs calculated using these data can be found in the associated paper [1]. Questions about the data or the limit calculations should be directed to [supercdms\\_publications@lists.astro.caltech.edu](mailto:supercdms_publications@lists.astro.caltech.edu).

## 1 Description of Files

### 1.1 Parameter Space

- *Mass\_charge\_bounds.txt*: This file contains the boundaries for mass vs charge parameter space for CDMSlite LIPs search analysis. LIPs have charge  $q = \pm fe$ , where  $e$  is the

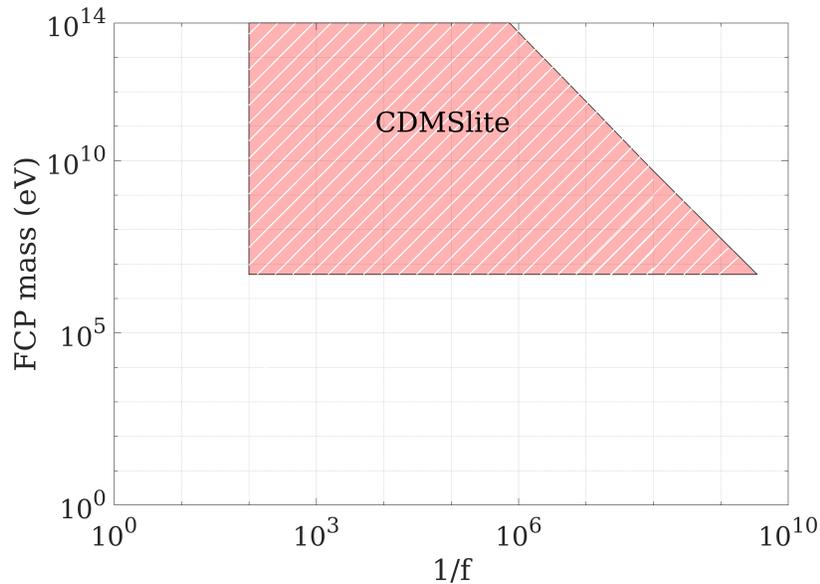

Figure 1: The mass vs charge parameter space for CDMSlite LIPs search analysis.

elementary charge and  $f$  has a value between 0 and 1. The first column consists of the

various  $f^{-1}$  values. The second and third columns consist of the lower mass bound and upper mass bound respectively. Figure 1 shows the mass versus charge parameter space of this analysis.

## 1.2 CDMSlite Run 2 Period 1 Data

- *EventEnergy\_keVee.txt*: This file contains a column of event energies in units of  $\text{keV}_{ee}$  from CDMSlite Run 2 Period 1. The energy range used in the LIP-search results is 0.1 to 2  $\text{keV}_{ee}$ ; the spectrum can be reproduced by using 190 bins of width 0.01  $\text{keV}_{ee}$  with the lowest energy bin spanning 0.1–0.11  $\text{keV}_{ee}$ . The file contains 180 events that pass all the selection criteria applied in the analysis. The spectrum generated is given in Fig. 2.

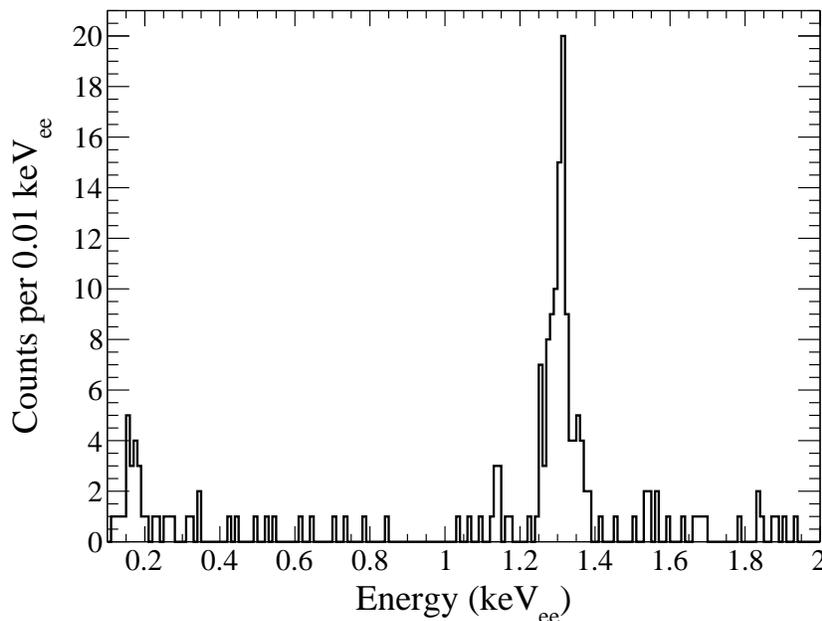

Figure 2: Energy spectrum of the CDMSlite Run2 Period1 data between 0.1  $\text{keV}_{ee}$  and 2  $\text{keV}_{ee}$ .

## 1.3 LIP Selection Efficiency

- *Efficiency\_CDMSlite\_Run2\_Period1.txt*: This file contains LIP-selection efficiency, along with  $\pm 1\sigma$  uncertainty, as a function of energies deposited in the detector for CDMSlite Run 2 Period 1. The data file has four columns; the description of each column is as follows.

Column 1: energies deposited in the detector,

Column 2: the efficiency at each energy,

Column 3: the  $1\sigma$  lower bound for each efficiency value, and

Column 4: the  $1\sigma$  upper bound for each efficiency value.

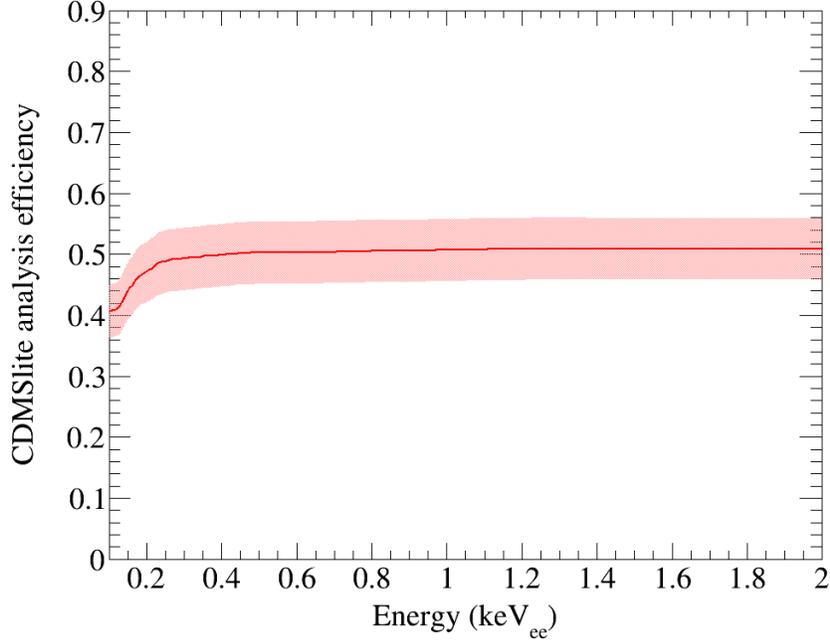

Figure 3: LIP selection efficiency along with  $\pm 1\sigma$  uncertainty on the efficiency values for energy depositions between  $0.1 \text{ keV}_{ee}$  and  $2 \text{ keV}_{ee}$ .

Figure 3 shows the LIP signal efficiency as a function of energy in the range  $0.1\text{--}2 \text{ keV}_{ee}$ . The  $\pm 1\sigma$  uncertainty band on the efficiency is also shown in the figure.

## 1.4 LIP Signal Model

- *CDMSlite\_LIP\_\*\_BetaGamma\_@\_#.txt*: The data to produce expected energy-deposition distributions for different charges and incident  $\beta\gamma$ <sup>1</sup> values is provided in these files. The energy-deposition distributions are calculated assuming isotropic or  $\cos^2\theta$  angular distributions for LIPs incident on the CDMSlite detector. In the file-names, “\*” refers to the  $f^{-1}$  values, “@” refers to the  $\beta\gamma$  values and “#” refers to the angular distributions (isotropic and  $\cos^2\theta$  distribution) of LIPs. Each data file has two columns: the first column is the energy deposition in eV and the second column is the probability density of energy deposition in the CDMSlite detector. The energy-deposition distributions are shown in Fig. 4.

## 1.5 LIP Efficiency Correction

- *LIPs\_efficiency\_correction.txt*: This file contains LIP-specific correction efficiency for various LIPs  $\beta\gamma$  value. This efficiency is energy dependent and its value only depends on the LIP-charge,  $\beta\gamma$  and assumed angular distribution. The uncertainty for all curves is smaller than 0.1%. The data file has seven columns; the description of each column is as follows:

---

<sup>1</sup> $\beta = v/c$  and  $\gamma = 1/\sqrt{1 - \beta^2}$ , where  $v$  is the LIP velocity.

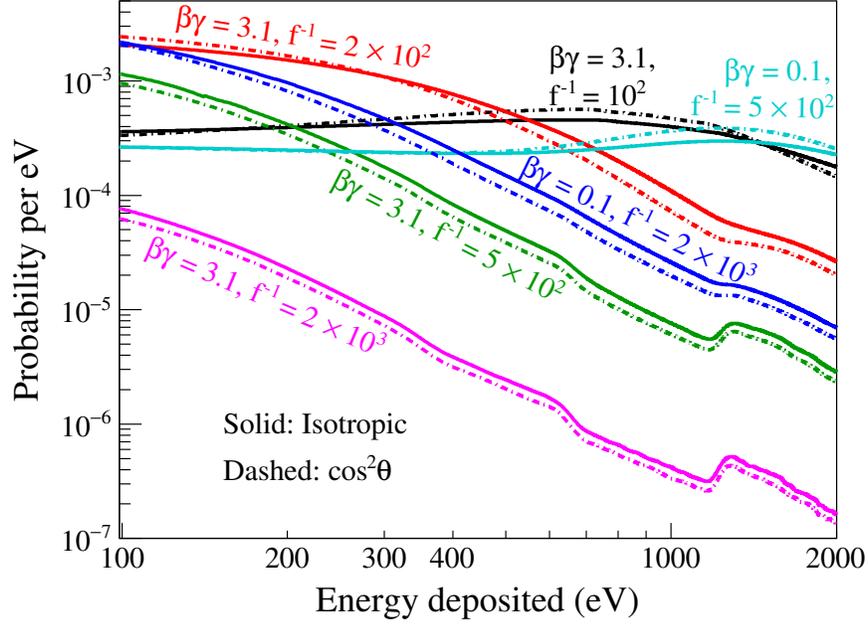

Figure 4: Simulated energy-deposition distributions averaged over incident angle for two different values of  $\beta\gamma$  and various  $f^{-1}$  between  $10^2$  and  $2 \times 10^3$ , after convolution with the detector energy resolution. The solid lines show the energy-deposition distributions assuming an isotropic incident LIP distribution, and the dash-dotted lines show the distribution assuming a  $\cos^2 \theta$  incident distribution.

Column 1: various inverse LIPs charges ( $f^{-1}$ ),

Column 2: LIPs efficiency correction factor for  $\beta\gamma$  value 0.1 assuming cosine squared angular distribution,

Column 3: LIPs efficiency correction factor for  $\beta\gamma$  value 0.1 assuming isotropic angular distribution,

Column 4: LIPs efficiency correction factor for  $\beta\gamma$  value 0.3 assuming isotropic angular distribution,

Column 5: LIPs efficiency correction factor for  $\beta\gamma$  value 1 assuming isotropic angular distribution,

Column 6: LIPs efficiency correction factor for  $\beta\gamma$  value 3.1 assuming isotropic angular distribution, and

Column 7: LIPs efficiency correction factor for  $\beta\gamma$  value 1000 assuming isotropic angular distribution.

Figure 5 shows the additional LIPs efficiency correction factors for various LIPs.

## 1.6 Intensity Limits

- *Intensity\_figure\_6.txt*: This file contains the limits on vertical intensity of LIPs for various LIPs  $\beta\gamma$ . The uncertainty band is only provided for  $\beta\gamma = 0.1$  but is indicative of the size

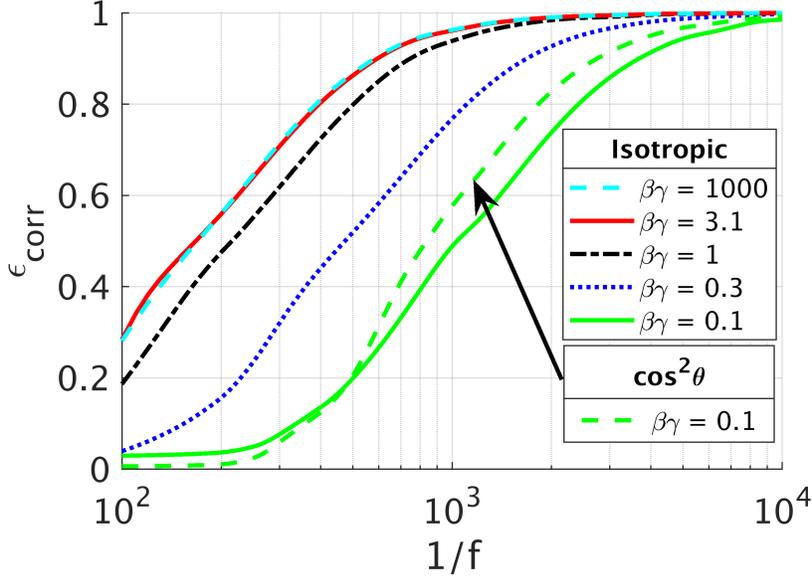

Figure 5: The LIP efficiency correction factor as a function of inverse LIP charge ( $f^{-1}$  for a variety of LIP  $\beta\gamma$ .

of the uncertainty of all the limit curves. The data file has nine columns; the description of each column is as follows:

Column 1: various inverse LIPs charges ( $f^{-1}$ ),

Column 2: the 90% confidence limit on vertical intensity for LIPs with different  $f^{-1}$  for  $\beta\gamma$  value 0.1 assuming an  $\cos^2\theta$  distribution,

Column 3: the 90% confidence limit on vertical intensity for LIPs with different  $f^{-1}$  for  $\beta\gamma$  value 1000 assuming an isotropic distribution,

Column 4: the 90% confidence limit on vertical intensity for LIPs with different  $f^{-1}$  for  $\beta\gamma$  value 3.1 assuming an isotropic distribution,

Column 5: the 90% confidence limit on vertical intensity for LIPs with different  $f^{-1}$  for  $\beta\gamma$  value 1.0 assuming an isotropic distribution,

Column 6: the 90% confidence limit on vertical intensity for LIPs with different  $f^{-1}$  for  $\beta\gamma$  value 0.3 assuming an isotropic distribution,

Column 7: the 90% confidence limit on vertical intensity for LIPs with different  $f^{-1}$  for  $\beta\gamma$  value 0.1 assuming an isotropic distribution,

Column 8: the lower limit of 1- $\sigma$  uncertainty on the intensity limit for LIPs  $\beta\gamma$  value 0.1 assuming isotropic distribution, and

Column 9: the upper limit of 1- $\sigma$  uncertainty on the intensity limit for LIPs  $\beta\gamma$  value 0.1 assuming isotropic distribution.

Figure 6 shows the 90 % confidence limit on LIP vertical intensity as a function of LIP electric charge for various values of LIP  $\beta\gamma$ .

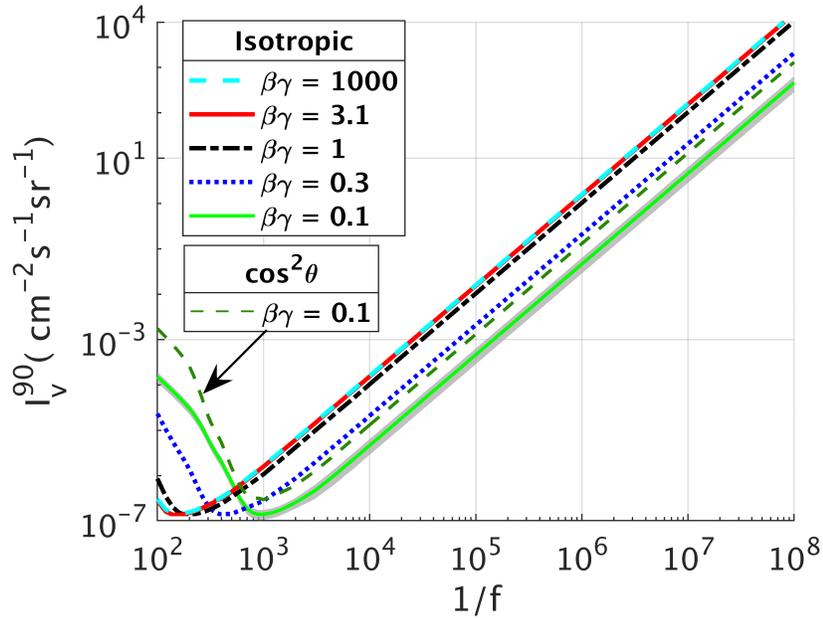

Figure 6: The 90 % confidence limit on LIP vertical intensity as a function of LIP electric charge for various values of LIP  $\beta\gamma$ . The limit curves for  $\beta\gamma \geq 10^3$  coincide with each other and are represented by a single curve. For clarity, the uncertainty band (light green) is only shown for  $\beta\gamma = 0.1$  but is indicative of the size of the uncertainty of all the limit curves.

## References

- [1] I. Alkhatib et al. (SuperCDMS Collaboration), Phys. Rev. Lett. 127, 081802.
